# Supplementary material for: Two-Port Feedback Analysis On Miller-Compensated Amplifiers
Source: arXiv:2207.10983 source file (2022-07-22)
Supplement: Supplementary file 1 [file Appendices_bk_0108.tex]

\appendices
\section{Two-port Feedback Analysis on Miller Compensated Two-stage Operational Amplifier}
\newcounter{mytempeqncnt}
\begin{figure*}[b]
\hrulefill
\vspace*{4pt}
\setcounter{mytempeqncnt}{\value{equation}} 
\setcounter{equation}{21}  
\begin{subequations} \label{ClTF1TF2}
\begin{align} 
H(s)& = \frac{-(R_{in}\parallel \frac{1}{s(C_{in}+C_c)})g_m(R_{o}\parallel \frac{1}{s(C_{o}+C_c)})}{1+ (R_{in}\parallel \frac{1}{s(C_{in}+C_c)})g_m(R_{o}\parallel \frac{1}{s(C_{o}+C_c)})sC_c}  \label{ClosedTF1}     \\ 
 & = -\frac{g_mR_{in}R_{o}}{1 + s[R_{in}C_{in} + R_{o}C_{o} + (g_mR_{in}R_{o} + R_{in} + R_{o})C_c] + s^2R_{in}R_{o}[C_{in}C_{o} + C_c(C_{in}+C_{o}) + C_c^2]} \label{ClosedTF2} 
\end{align}
\end{subequations}
\begin{subequations} \label{ClTF3TF4}
\begin{align} 
H_{\textrm{direct}}(s)& =  -\frac{(g_m-sC_c)R_{in}R_{o}}{1 + s[R_{in}C_{in} + R_{o}C_{o} + (g_mR_{in}R_{o} + R_{in} + R_{o})C_c] + s^2R_{in}R_{o}[C_{in}C_{o} + C_c(C_{in}+C_{o})]} \qquad \qquad    \label{ClosedTF3}  \\ 
 & = \frac{-(R_{in}\parallel \frac{1}{s(C_{in}+C_c)})(g_m-sC_c)(R_{o}\parallel \frac{1}{s(C_{o}+C_c)})}{1+ (R_{in}\parallel \frac{1}{s(C_{in}+C_c)})(g_m-sC_c)(R_{o}\parallel \frac{1}{s(C_{o}+C_c)})sC_c}  \label{ClosedTF4}
\end{align}
\end{subequations}
\setcounter{equation}{\value{mytempeqncnt}}
\end{figure*}

\begin{figure}[t]
\centering
\includegraphics[width=3.45in]{Figs/FigApp1}
\caption{(a) Traditional Miller-compensated two-stage op-amp. (b) Feedback amplifier with a shunt-shunt feedback topology. (c) Small-signal model of the $A$ circuit with the definition of $a(s)$ and $a'(s)$. (d) Small-signal model of the $\beta$ circuit with the definition of $\beta(s)$.}
\label{FigApp1}
\end{figure}
The traditional Miller-compensated two-stage op-amp is analyzed using the two-port feedback analysis (TFA)~\cite{Sedra} here. The circuit is shown in Fig.~\ref{FigApp1}(a). The transconductance, lumped resistance, and capacitance at the input $v_{in}$ node (at the output $v_{o}$ node) are modeled as $g_m$, $R_{in}$ ($R_{o}$), $C_{in}$ ($C_{o}$), respectively. Also, $i_{s}$ represents the input signal current to the circuit, and $C_c$ represents a compensating capacitor. The circuit can be considered a feedback amplifier having a shunt-shunt feedback topology as illustrated in Fig.~\ref{FigApp1}(b); the basic amplifier is a unilateral trans-impedance amplifier, and the feedback network is the compensating capacitor that samples the output voltage $v_{o}$, and provides the feedback current $i_{f}$ subtracted from the input signal current $i_{s}$ at the input node. Thus, we apply the rules of the corresponding two-port feedback analysis to find its $A$ circuit, and $\beta$ circuit, giving forward transfer function $a(s)$, and feedback transfer function $\beta(s)$, respectively.

Fig.~\ref{FigApp1}(c) shows the small-signal model of the $A$ circuit with its input current $i_{in}$ including a loading effect of the feedback network, and its associated forward transfer function before ($a(s)$), and after ($a'(s)$) shunting a current source $sC_cv_{in}$ at the output node that reflects the feedforward current through $C_c$, respectively. That signal feedforward transmission through the feedback network, and thus a resulting right-half-plane (RHP) zero, are ignored in the following analysis; however, the analysis including the effect of the RHP zero will be dealt later. 

The forward transfer function $a(s)$ can be easily found by inspection due to its open-loop characteristic, and is given by
\begin{align}
a(s) & \equiv   \frac{v_o(s)}{i_{in}(s)} \nonumber \\ 
& =  -(R_{in}\parallel \frac{1}{s(C_{in}+C_c)})g_m(R_{o}\parallel \frac{1}{s(C_{o}+C_c)}) \nonumber \\ 
& = -\frac{g_mR_{in}R_{o}}{[1+sR_{in}(C_{in}+C_c)][1+sR_{o}(C_{o}+C_c)]} \label{eq3} 
\end{align}
where $X\parallel Y = XY/(X+Y)$. From~(\ref{eq3}), $a(s)$ has two left-half-plane (LHP) real poles given by
\begin{subequations} \label{pinandpo}
\begin{align} 
p_{in} & = -\frac{1}{R_{in}(C_{in}+C_c)}  \label{pin}  \\
p_{o} &  = -\frac{1}{R_{o}(C_{o}+C_c)}.    \label{po}
\end{align}
\end{subequations}
Fig.~\ref{FigApp1}(d) shows the small-signal model of the $\beta$ circuit, and its associated feedback transfer function $\beta(s)$ is given by
\begin{align}
\beta(s) \equiv \frac{i_f(s)}{v_{o}(s)} = -sC_c \label{betafunc} 
\end{align}
From~(\ref{betafunc}), $\beta(s)$ has a zero $z_{\beta}$ at the origin (i.e., $z_{\beta} = 0$). 

Combining (\ref{eq3}) and (\ref{betafunc}), the $a(s)\beta(s)$ is expressed as

\begin{align}
 a(s)\beta(s) = \frac{g_mR_{in}R_{o}C_cs}{[1+sR_{in}(C_{in}+C_c)][1+sR_{o}(C_{o}+C_c)]}. \label{LT1} 
\end{align}

Substituting~(\ref{eq3}), (\ref{LT1}) into the feedback equation~$H(s) = a(s)/(1+a(s)\beta(s))$, and following some algebraic manipulation, the closed-loop transfer function $H(s) = v_o(s)/i_s(s)$ can be found as~(\ref{ClTF1TF2}) shown at the bottom of the page. The exact closed-loop transfer function $H_{\textrm{direct}}(s)$ is also shown as~(\ref{ClTF3TF4}) obtained by the direct analysis to investigate the validity of the two-port feedback analysis. Comparing~(\ref{ClosedTF1}) with (\ref{ClosedTF4}) shows that the only difference is that $g_m$ has been replaced by ($g_m - sC_c$). This difference stems from the feedforward through $C_c$ that results in a generation of a RHP zero $z_{RHP}= g_m/C_c$ which provides the closed-loop transfer function with a proper sign reversal at DC when plotted in the $s$-plane, and a magnitude-extension of the non-dominant pole by subtracting ${C_c}^2$ from the coefficient of $s^2R_{in}R_o$ in the denominator of (\ref{ClosedTF2}), yielding~(\ref{pndRHP}).\footnote{For this reason, if the effect of the signal feedforward through the feedback network is assumed to be neglected, the denominator of (\ref{ClosedTF2}) should be investigated rather than that of (\ref{ClosedTF3}) to find the poles of the closed-loop transfer function.} That feedforward was assumed to be ignored in the analysis here; (\ref{ClosedTF4}) can be also obtained by the two-port feedback analysis with the forward transfer function $a'(s)$, rather than $a(s)$. Thus, the analysis here is reasonably accurate if $g_m \gg \abs{sC_c}$ at the frequencies of interest.

\begin{figure}[t]
\centering
\includegraphics[width=3.45in]{Figs/FigApp2}
\caption{Root-locus diagram for (\ref{LT1}), and the pole-splitting relation.}
\label{FigApp2}
\end{figure}
The poles of the $H(s)$ is found by drawing the root-locus diagram shown in Fig.~\ref{FigApp2} rather than by directly factoring the denominator of (\ref{ClosedTF2}). It includes the both cases that the $p_{d,init}=p_{in}$ (i.e., $R_{in}(C_{in}+C_c) > R_{o}(C_{o}+C_c)$), and the $p_{d,init}=p_{o}$ (i.e., $R_{o}(C_{o}+C_c) > R_{in}(C_{in}+C_c)$). The resulting diagram shows important facts: 

(1) Regardless of the condition about the $p_{d,init}$ location, the diagram shows the two initial poles must always be splitted as $L_{MID}$ increases; $p_{d,init} \rightarrow 0^-$, $p_{nd,init} \rightarrow -\infty$ as $L_{MID} \rightarrow \infty$; it agrees with~\cite{WHKi}. 

(2) It also predicts that the closed-loop transfer function has only the two real LHP poles since the $z_\beta$ at the origin is a phantom zero, and $a(s)$ has no zeros; it can be confirmed by~(\ref{ClosedTF2}).

(3) The locations of the closed-loop dominant ($p_d$), and non-dominant ($p_{nd}$) poles can be found as follows: (\ref{LT1}) can be written in the form  

\begin{figure}[t]
\centering
\includegraphics[width=3.45in]{Figs/FigApp3}
\caption{A Bode magnitude plot for $L(s)$ when the $p_{d,init}$ is either (a)~$p_{in}$, or (b)~$p_o$. Note that $L_{MID}$ is different in each case.}
\label{FigApp3}
\end{figure}

\addtocounter{equation}{2}
\begin{align*}
 a(s)\beta(s) = \frac{L_{MID}\frac{s}{\abs{p_{d,init}}}}{(1+\frac{s}{\abs{p_{d,init}}})(1+\frac{s}{\abs{p_{nd,init}}})}. 
\end{align*}
Assuming $L_{MID} \gg 1$, the zeros of the characterisitic equation $1 + a(s)\beta(s)$ can be approximately found by solving the following polynomial  
\begin{align}
D(s)  = 1+s\frac{L_{MID}}{\abs{p_{d,init}}} +s^2\frac{1}{\abs{p_{d,init}}\abs{{p_{nd,init}}}}.  \label{LT3} 
\end{align}
If the two roots of $D(s)$ are real and widely spaced (i.e., $\abs{p_{nd}} \gg \abs{p_d}$) , which is typically true, then
\begin{align}
D(s) \simeq 1+s\frac{1}{\abs{p_{d}}} +s^2\frac{1}{\abs{p_{d}}\abs{{p_{nd}}}}.  \label{LT4} 
\end{align}
Equating the coefficient of $s$ in~(\ref{LT3}) and in~(\ref{LT4}) results in 
\begin{align}
\abs{p_d} \simeq \frac{\abs{p_{d,init}}}{L_{MID}}.  \label{pd} 
\end{align}
Similarly, the $p_{nd}$ can be estimated by equating coefficients of $s^2$ in~(\ref{LT3}) and in~(\ref{LT4}), and using~(\ref{pd}).
\begin{align}
\abs{p_{nd}} \simeq L_{MID} \abs{p_{nd,init}}.  \label{pnd} 
\end{align}
Using (\ref{pd}), (\ref{pnd}), we can establish a following simple \textbf{pole-splitting relation}: 
\begin{equation}
  \boxed{L_{MID}  \simeq \frac{p_{d,init}}{p_d}  \simeq \frac{p_{nd}}{p_{nd,init}}}. \label{PoleSplit}
\end{equation}
Using the pole-splitting relation, the locations of the closed-loop poles for any system whose loop-transmission has two LHP real poles and a zero at the origin can be easily obtained. Depending on the condition whether the $p_{d,init} = p_{in}$ or $p_{d,init} = p_{o}$, $L_{MID}$s are differently expressed as 
\begin{equation}
    L_{MID} = 
    \begin{cases}
    \begin{split}
      \frac{g_mR_oC_c}{C_{in}+C_c} &  \,\,\,\, \text{if } p_{d,init} = p_{in}     \\
      \frac{g_mR_{in}C_c}{C_o+C_c} &  \,\,\,\, \text{if } p_{d,init} = p_{o}   \label{LMID}
    \end{split}
    \end{cases}
\end{equation}
and both cases are graphically illustrated as shown in Fig.~\ref{Fig5}(a), (b), respectively. Substitution of~(\ref{pinandpo}) and (\ref{LMID}) into (\ref{PoleSplit}) gives
\begin{equation}
p_{d}  \simeq -\frac{1}{g_mR_{in}R_oC_c}  \label{pd2} 
\end{equation}
\begin{equation}
p_{nd} \simeq -\frac{g_mC_c}{(C_{in}+C_c)(C_o+C_c)}.    \label{pnd2}
\end{equation}
These poles are the same with those obtained by approximately solving the denominator of~(\ref{ClosedTF2}), and are illustrated in Fig.~\ref{Fig4}.

(\ref{pd2}), (\ref{pnd2}) are also the poles of the input ($Z_{in}(s)$), and the output ($Z_{o}(s)$) impedance of the circuit because the poles of the circuit does not be affected by an excitation source that does not change its natural structure~\cite{Sedra}. However, the location of the zero is different; $Z_{in}(s)$ is defined as $v_{in}(s)/i_{s}(s)$ in Fig.~\ref{FigApp1}(a), modifying its $A$ circuit to yield a forward transfer function as $v_{in}(s)/i_{in}(s)$ in Fig.~\ref{FigApp1}(c), and its $\beta$ circuit to yield a feedback transfer function as $i_{f}(s)/v_{in}(s) = (v_{o}(s)/v_{in}(s))\beta(s)$ in Fig.~\ref{FigApp1}(c), (d). That implies the feedback path has a pole at $s=p_o$, generating a zero at the same location in $Z_{in}(s)$. Similarly, the $Z_{o}(s)$ can be determined by removing $i_{s}(s)$ at $v_{in}$ node, and shunting an independent test current source $i_{t}(s)$ at $v_o$ node, and analyzing the $v_{o}(s)/i_{t}(s)$ in Fig.~\ref{FigApp1}(a); then, its feedback path has a pole at $s=p_{in}$, generating a zero at the same location in $Z_{o}(s)$. Note that $\beta(s)$ is in the feedback path in both cases, and thus $z_{\beta}$ at the origin is the phantom zero.

\begin{figure}[t]
\centering
\includegraphics[width=3.45in]{Figs/FigApp4}
\caption{Pole-zero diagram with its DC magnitude for (a) $H(s)$, (b) $Z_{in}(s)$, and (c) $Z_{o}(s)$.}
\label{FigApp4}
\end{figure}

The pole-zero diagrams for $A(s)$, $Z_{in}(s)$, and $Z_{o}(s)$ are shown in Fig.~\ref{Fig6}(a), (b), and (c), respectively. Note that in each diagram its DC value is also depicted which can be easily obatined by inspection; thus, its associated Bode plot can be drawn trivially. 

It is worth mentioning that if the system is positive feedback system (i.e., if $-g_m$ in Fig.~\ref{FigApp1}(a) is replaced with $+g_m$), then the root-locus diagram would be drawn with negative locus rules applied; the two intial poles attracts each other, rather than splitted, as $L_{MID}$ increases, and forms complex-conjugate pole-pair when $L_{MID}$ is larger than some finite value at which the two LHP poles coincides. This observation may provide insights to design high $Q$ filters using positive feedback such as the Sallen-Key circuits~\cite{Sallen}.

Fig.~\ref{Fig3}(c) also shows the $A$ circuit including a loading effect of the feedback network, and its associated forward transfer function $a'(s)$ after adding a current source $sC_cv_{in}$ that reflects the feedforward current thorugh $C_c$, respectively. $a'(s)$ can be found easily by inspection, and is given by
\begin{align}
a'(s)  \equiv  \frac{v'_o(s)}{i_{in}(s)}  = -\frac{g_mR_{in}R_{o}(1-\frac{s}{z_{RHP}})}{(1+\frac{s}{\abs{{p_{in}}}})(1+\frac{s}{\abs{{p_{o}}}})}	\label{aprimefunc}	
\end{align}
\noindent where $p_{in}$, $p_{o}$ are expressed as (\ref{pin}), (\ref{po}), respectively, and $z_{RHP} = g_m/C_c$.

(\ref{aprimefunc}) combined with~(\ref{betafunc}) yields the the $a'(s)\beta(s)$ is expressed as
\begin{align}
   a'(s)\beta(s) = \frac{g_mR_{in}R_{o}C_cs(1-\frac{s}{z_{RHP}})}{(1+\frac{s}{\abs{{p_{in}}}})(1+\frac{s}{\abs{{p_{o}}}})} \label{aprimebeta} 
\end{align}

Substituting~(\ref{aprimefunc}), (\ref{aprimebeta}) into the the feedback equation~$H'(s) = a'(s)/(1+a'(s)\beta(s))$, and following some algebraic manipulation, the closed-loop transfer function $H'(s) = v'_o(s)/i_s(s)$ is given by~(\ref{ClosedTF4}) which is exactly the same with~(\ref{ClosedTF3}) obtained by the direct analysis, strictly validating the two-port analysis.

Before the root locus diagram for~(\ref{aprimebeta}) is drawn, a special care must be given \cite{Roberge}; since (\ref{aprimebeta}) does not reflect the sign reversal at $s = 0^+$ associated with the $z_{RHP}$ when plotted in the $s$-plane, it should be slightly modified as 
\begin{align}
   \textrm{Modified} \,\, a'(s)\beta(s) = \frac{-g_mR_{in}R_{o}C_cs(1-\frac{s}{z_{RHP}})}{(1+\frac{s}{\abs{{p_{in}}}})(1+\frac{s}{\abs{{p_{o}}}})}. \label{aprimebetaMod} 
\end{align}
Since (\ref{aprimebetaMod}) has a negative sign at its midband frequency, the system is now considered a positive feedback system. Thus, root locus diagram is drawn with negative locus rules applied is shown in Fig.~\ref{FigApp5}. 

The diagram shows the two initial poles must always be splitted as $L_{MID}$ increases, regardless of the condition about the $p_{d,init}$ location as in the case that the signal feedforward thorugh $C_c$ is ignored. Also, the diagram also predicts that the closed-loop transfer function $A'(s) = v'_o(s)/i_s(s)$ has the two real LHP poles ($p_{d}$, $p_{nd}$), and a zero in RHP ($z_{RHP}$) since the $z_\beta$ at the origin is a phantom zero, and the $z_{RHP}$ stems from $a'(s)$; it can be confirmed by~(\ref{ClosedTF3}).

To determine the closed-loop poles locations, the pole-splitting relation (\ref{PoleSplit}) cannot be blindly applied here, because (\ref{PoleSplit}) has been derived from the loop-transmission that has the two LHP poles and a zero at the origin. However, the resulting pole locations can be described intuitively through nonrigorous terms as follows. $\abs{p_{d,init}},\abs{p_{nd,init}}$ are typically much smaller than $z_{RHP}$ because $z_{RHP}$ is linearly proportinal to $g_m$. Therefore, $z_{RHP}$ has little effect on the loop-transmission magnitudes at the frequencies $\omega = \abs{p_{d,init}}, \abs{p_{nd,init}}$ . Thus, $p_d$, which is located at much lower frequency than $p_{d,init}$, is the same with~(\ref{pd}). However, as $p_{nd,init}$ goes to higher frequency, its magnitude is becoming comparable to that of $z_{RHP}$. This zero increases the loop-transmission magnitude at the high frequency, causing the closed-loop non-dominant pole to be located at a higher frequency than (\ref{pnd}).

Such extension of the non-dominant pole can also be explained using the root-locus diagram shown in Fig.~\ref{FigApp5}. As $L_{MID} \rightarrow \infty$, $p_{nd,init} \rightarrow z_{RHP}^+$, implying $p_{nd}$ can be located at nearer to the $-\infty$ than the case without $z_{RHP}^+$ at the finite $L_{MID}$ applied. It can be verified by factoring the denominator of (\ref{ClosedTF4}), apprixmiately yielding the dominant pole as the same with~(\ref{pd}), and the non-domiant pole as 

\begin{equation}
p_{nd} \simeq -\frac{g_mC_c}{(C_{in}+C_c)(C_o+C_c)-{C_c}^2}.   \label{pndRHP}
\end{equation}
whose magnitude is obviously larger than that of~(\ref{pnd2}). 
\begin{figure}[t]
\centering
\includegraphics[width=3.45in]{Figs/FigApp5}
\caption{Root-locus diagram for (\ref{aprimebetaMod}) with negative locus rules applied.}
\label{FigApp5}
\end{figure}

% you can choose not to have a title for an appendix
% if you want by leaving the argument blank
\section{Zeros for Gain of PTAT Embedded Amplifier}
The PTAT embedded amplifier with internal cascode devices $M_{2L,R}$ neglected for simplicity is shown in Fig.~\ref{FigApp6}. Since the size of $M_1$ is much larger than that of other devices, a gate-to-drain capacitance of $M_1$ ($C_{gd}$) is included here. The current $i_{\textrm{x}}$ is the drain current of $M_\textrm{x}$, $i_{o1}$ is the amplifier output current, $i_{ff}$ is the feedforward current from $v_{in}$ to $v_{o1}$ through $C_{gd}$, and the arrows indicate their directions. The output capacitor $C_{o1}$ and the equivalent single-ended compensating capacitor $C_c$ are attached at $v_{o1}$, and $v_c$ nodes, respectively. 

At zeros of the amplifier gain transfer funcition, $v_{o1} = 0$. Thus, there is no current flow into $C_{o1}$ (i.e., $i_{o1} = 0$.). Then, the locations of the zeros can be obatined by applying KCL at $v_{o1}$ node with $i_{o1} = 0$. Assuming an infinite output resistance of the tail current source and $g_{m1L} = g_{m1R} \equiv g_{m1}$ for simplicity, we can write 
\begin{align*}
i_{1L} & = -i_{1R} = -\frac{g_{m1L}g_{m1R}v_{in}}{g_{m1L}+g_{m1R}}   \\
i_{3L} & = -i_{1R}\frac{g_{m3L}}{g_{m3R}+sC_c} = -\frac{g_{m1L}g_{m1R}g_{m3L}v_{in}}{(g_{m1L}+g_{m1R})(g_{m3R}+sC_c)}  \\
i_{ff} & = sC_{gd}v_{in}.  
\end{align*}
Solving $i_{1L} + i_{3L} + i_{ff} = 0$ with some algebraic manipulations result in the zeros of the amplifier are the roots of  
\begin{equation*}
2C_{gd}C_cs^2 + (2C_{gd}g_{m3R}-C_cg_{m1})s - g_{m1}(g_{m3L}+g_{m3R}) = 0.  \label{zeroroot}
\end{equation*}
Thus, there are two zeros located at RHP ($z_2$), and at LHP ($z_3$) as given by 
\begin{align}
z_{2,3}  = \frac{g_{m1}}{4C_{gd}}-\frac{g_{m3R}}{2C_{c}} \pm \frac{\sqrt{\Delta}}{4C_cC_{gd}}  \label{z22} 
\end{align}
where $\Delta=$
\begin{align*}
C_c^2g_{m1}^2+4C_cC_{gd}g_{m1}g_{m3R}+8C_cC_{gd}g_{m1}g_{m3L}+4C_{gd}^2g_{m3R}^2. 
\end{align*}
When $g_{m1}/4C_{gd} < g_{m3R}/2C_{c}$ that is the case in the proposed BGR, $\abs{z_3} > \abs{z_2}$ as shown in Fig.~\ref{Fig7}(a).

\begin{figure}[t]
\centering
\includegraphics[width=2.45in]{Figs/FigApp6}
\caption{Simplified PTAT embedded amplifier to investigate zero locations.}
\label{FigApp6}
\end{figure}
